# Supplementary material for: Accelerating and enhancing thermodynamic simulations of electrochemical interfaces
Source: arXiv:2503.17870 ancillary file (2025-03-22)
Supplement: Supplementary file 1 [file SI.pdf]

# Supporting Information for: Accelerating and enhancing thermodynamic simulations of electrochemical interfaces

Xiaochen Du,† Mengren Liu,‡ Jiayu Peng,‡ Hoje Chun,‡ Alexander Hoffman,‡ Bilge Yildiz,‡,¶ Lin Li,§ Martin Z. Bazant,† and Rafael Gómez-Bombarelli*,‡

†*Department of Chemical Engineering, Massachusetts Institute of Technology, Cambridge, MA 02139, USA*

‡*Department of Materials Science and Engineering, Massachusetts Institute of Technology, Cambridge, MA 02319, USA*

¶*Department of Nuclear Science and Engineering, Massachusetts Institute of Technology, Cambridge, MA 02319, USA*

§*Massachusetts Institute of Technology Lincoln Laboratory, Lexington, MA, 02421, USA*

E-mail: rafagb@mit.edu

## Abbreviations used

- CHE: Computational hydrogen electrode
- DFT: Density-functional theory
- GCMC: Grand-canonical Monte Carlo
- GGA: Generalized-gradient approximation
- GMM: Gaussian mixture model

- MAE: Mean-absolute error
- MC: Monte Carlo
- ML: Machine learning
- NFF: Neural network force field
- OER: Oxygen evolution reaction
- ORR: Oxygen reduction reaction
- PAW: Projector augmented-wave
- PBE: Perdew-Burke-Ernzerhof (functional)
- PC: Principal component
- SD: Standard deviation
- SHE: Standard hydrogen electrode
- VASP: Vienna *ab initio* Simulation Package
- VSSR-MC: Virtual Surface Site Relaxation-Monte Carlo

## Supplementary figures

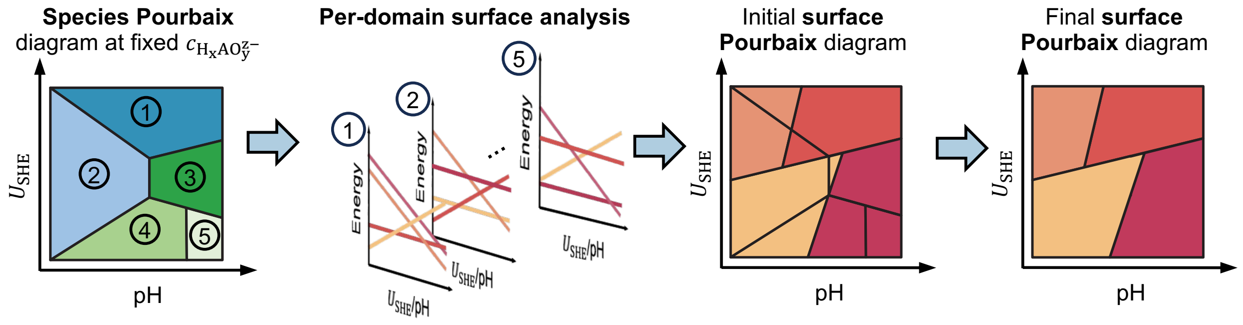


Figure S1: **Schematic for conventional surface Pourbaix diagram at fixed** $c_{H_xAO_y^{z-}}$**.** Separate $\Omega_{slab}(U_{SHE}, pH)$ is considered for each surface in each species domain. Individual convex hull analyses yield stable surface domains for each species domain. Merging identical surface domains results in the final surface Pourbaix diagram.

.

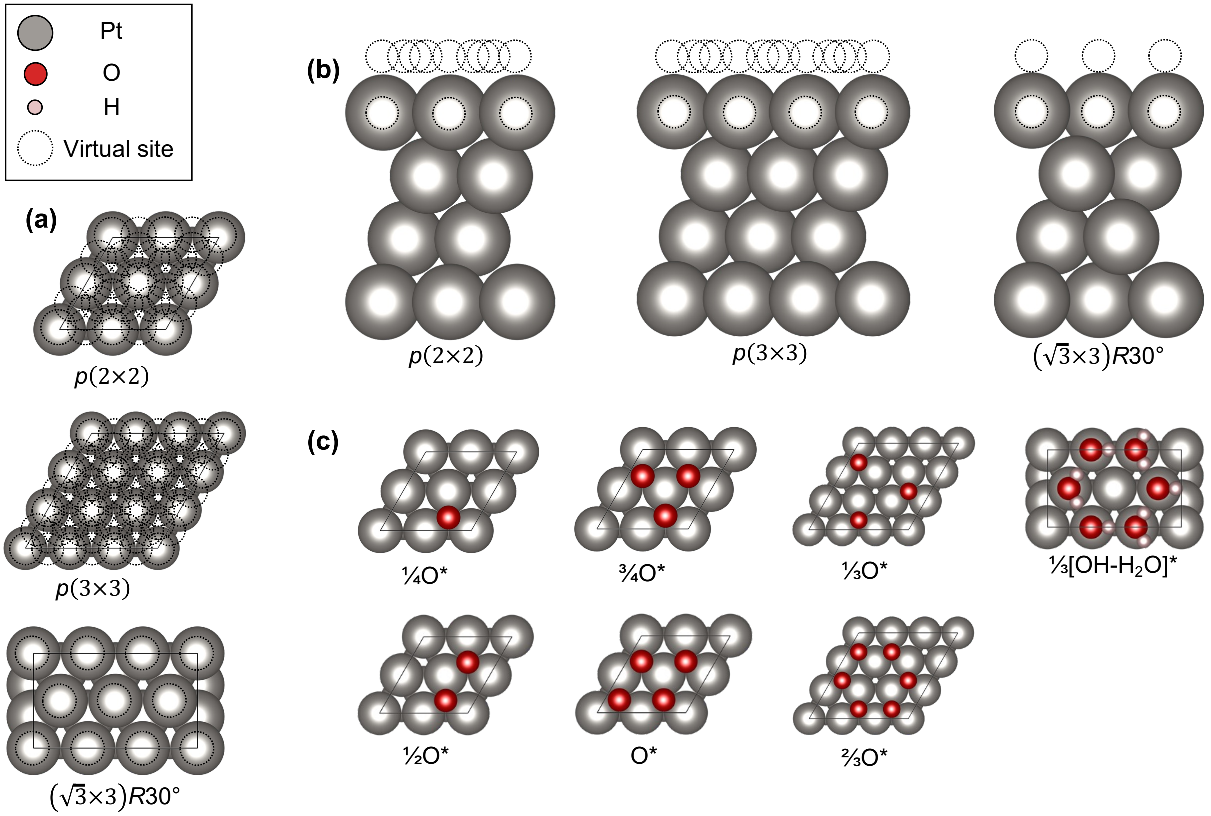


Figure S2: **Set of literature surfaces used in Pt(111) surface analysis.** (a) Top-down view of $(\sqrt{3}\times 3)$R30°, $p(2\times 2)$, and $p(3\times 3)$ pristine surfaces and virtual sites used for VSSR-MC sampling. (b) Side view of pristine surfaces and virtual sites. The pristine surface layer is included in the virtual sites. (c) Handpicked reconstructions obtained from Hansen *et al.*[1] and Vinogradova *et al.*[2]

.

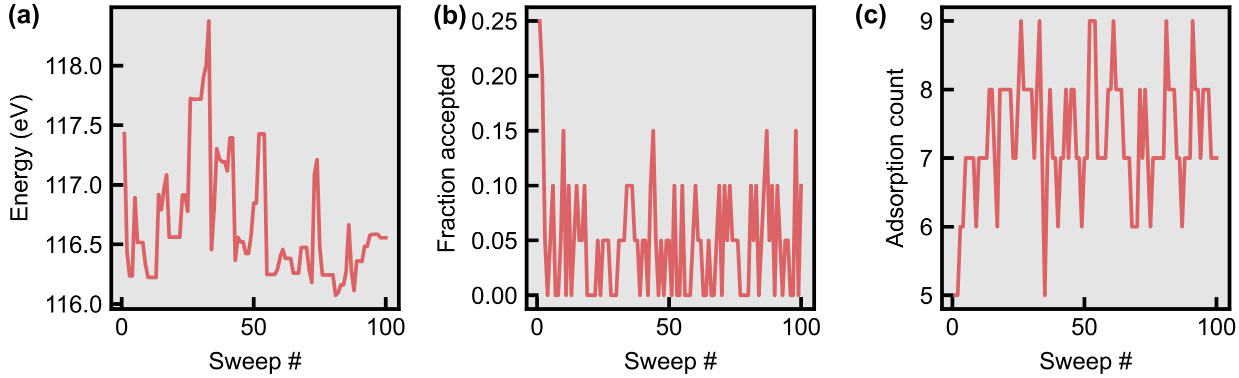


Figure S3: **VSSR-MC sampling profile for** $p(3\times 3)$ **Pt(111) at pH = 8,** $U_{\mathbf{SHE}}$ **= 1.0 V.** (a) Surface Pourbaix grand potential ($\Omega_{\text{slab}}(U_{\text{SHE}}, \text{pH})$) energy evaluated using pre-trained CHGNet, (b) fraction of MC iterations accepted, and (c) number of adsorbed atoms. Each sweep consists of 20 MC sampling iterations.

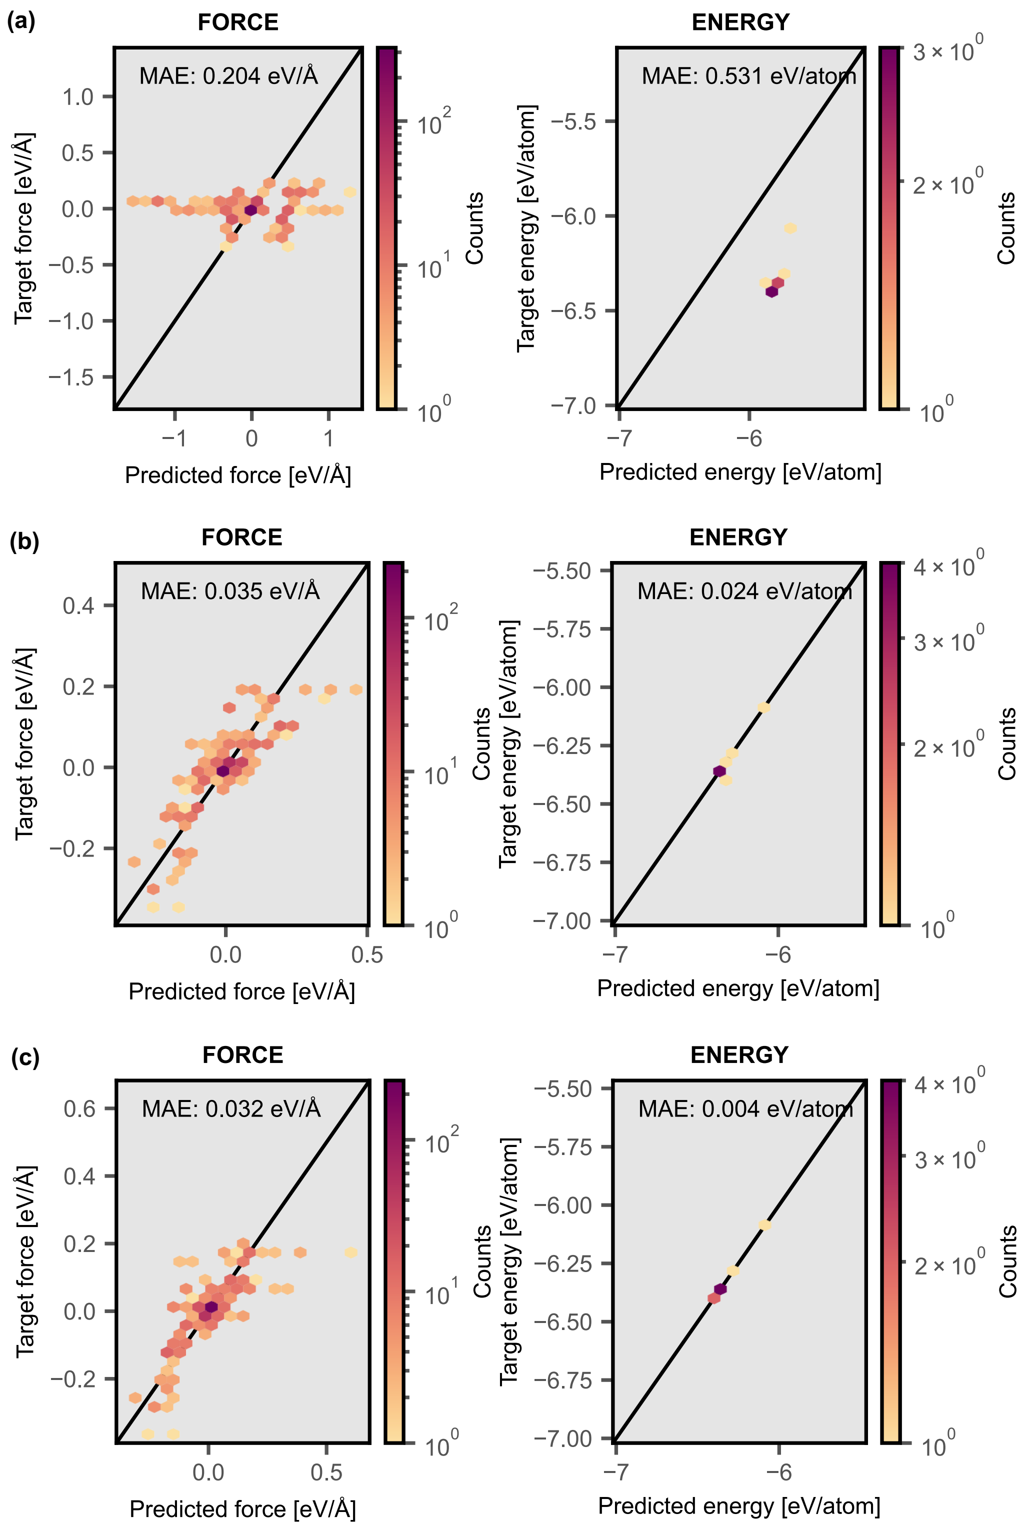


Figure S4: **NFF performance comparison for Pt(111) on the 8 handpicked surfaces.** (a) pre-trained CHGNet, (b) fine-tuned CHGNet, and (c) fine-tuned MACE.

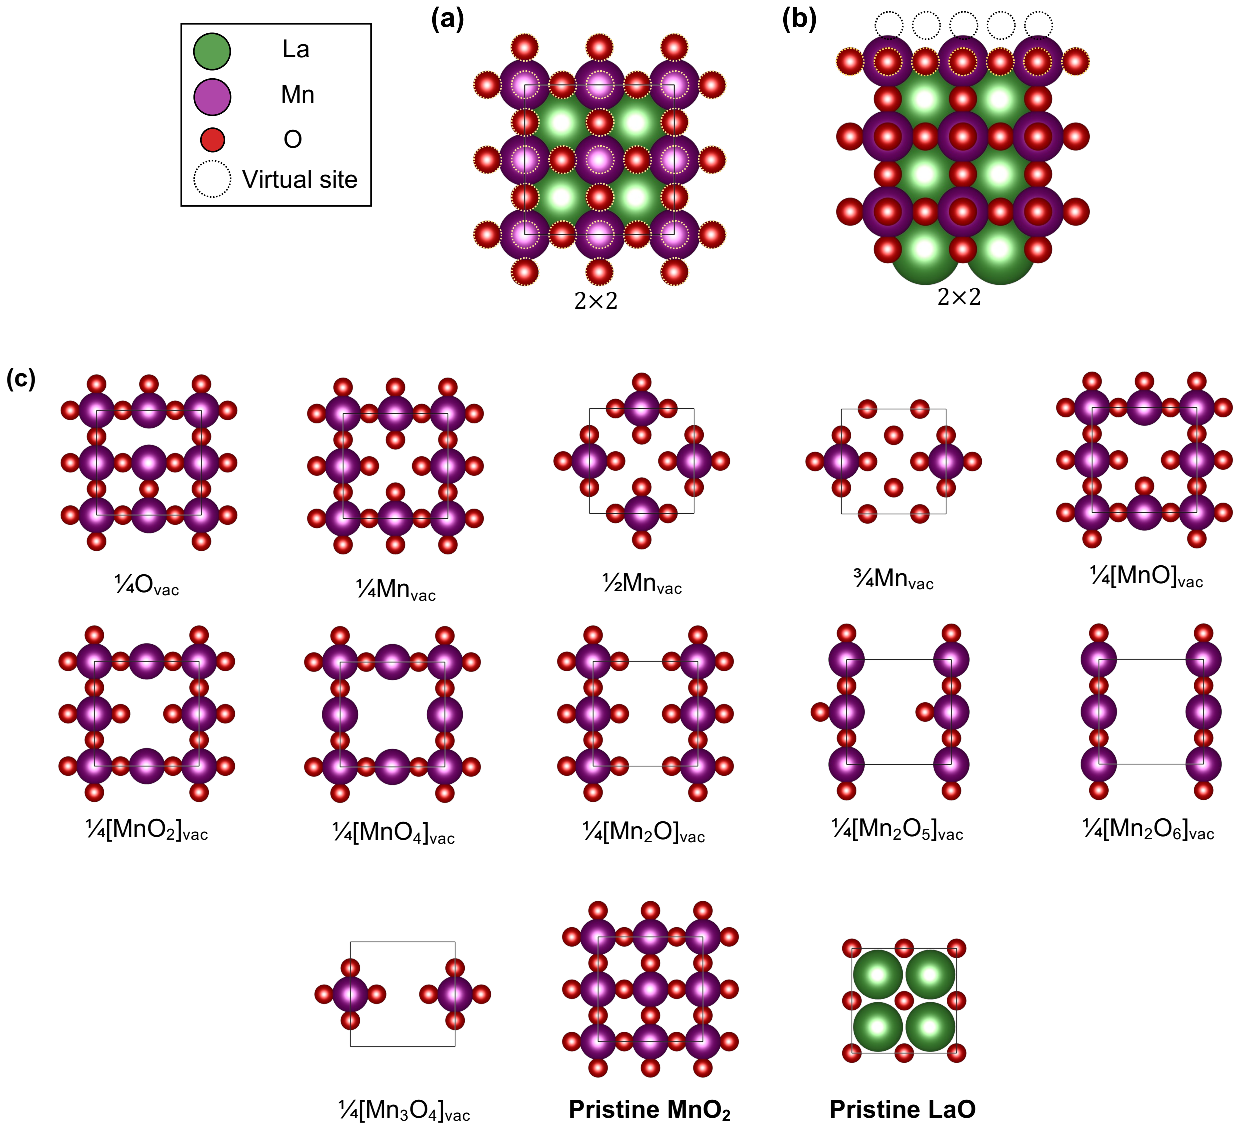


Figure S5: **Set of literature surfaces used in $LaMnO_3$(001) surface analysis.** (a) Top-down view of $2 \times 2$ pristine surface and virtual sites used for VSSR-MC sampling. (b) Side view of pristine surface and virtual sites. The pristine surface layer is included in the virtual sites. (c) Handpicked reconstructions obtained from Rong and Kolpak.[3] Additional surfaces with varying coverages of O* and OH* were also included for a total of 47 structures.[4]

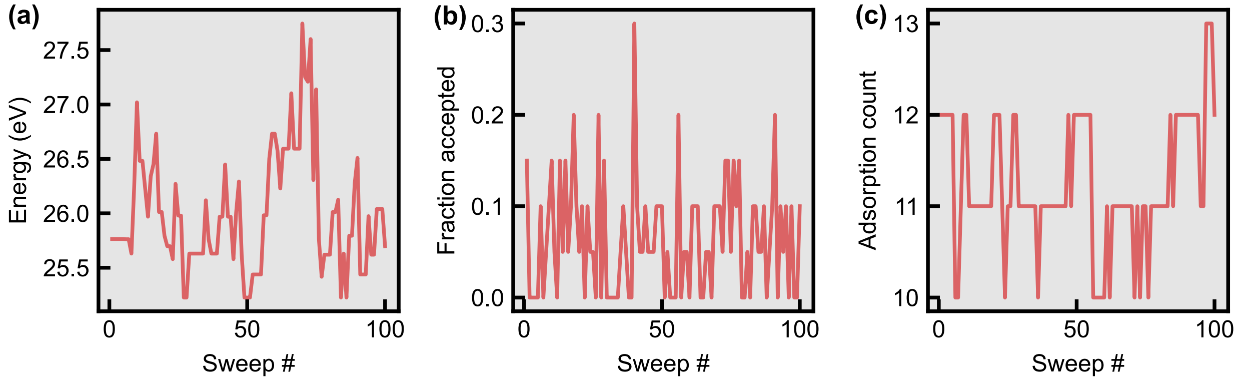


Figure S6: **VSSR-MC sampling profile for $2 \times 2$ LaMnO$_3$(001) at pH = 10, $U_{\text{SHE}}$ = 1.0 V.** (a) Surface Pourbaix grand potential ($\Omega_{\text{slab}}(U_{\text{SHE}}, \text{pH})$) energy evaluated using pre-trained CHGNet, (b) fraction of MC iterations accepted, and (c) number of adsorbed atoms. Each sweep consists of 20 MC sampling iterations.

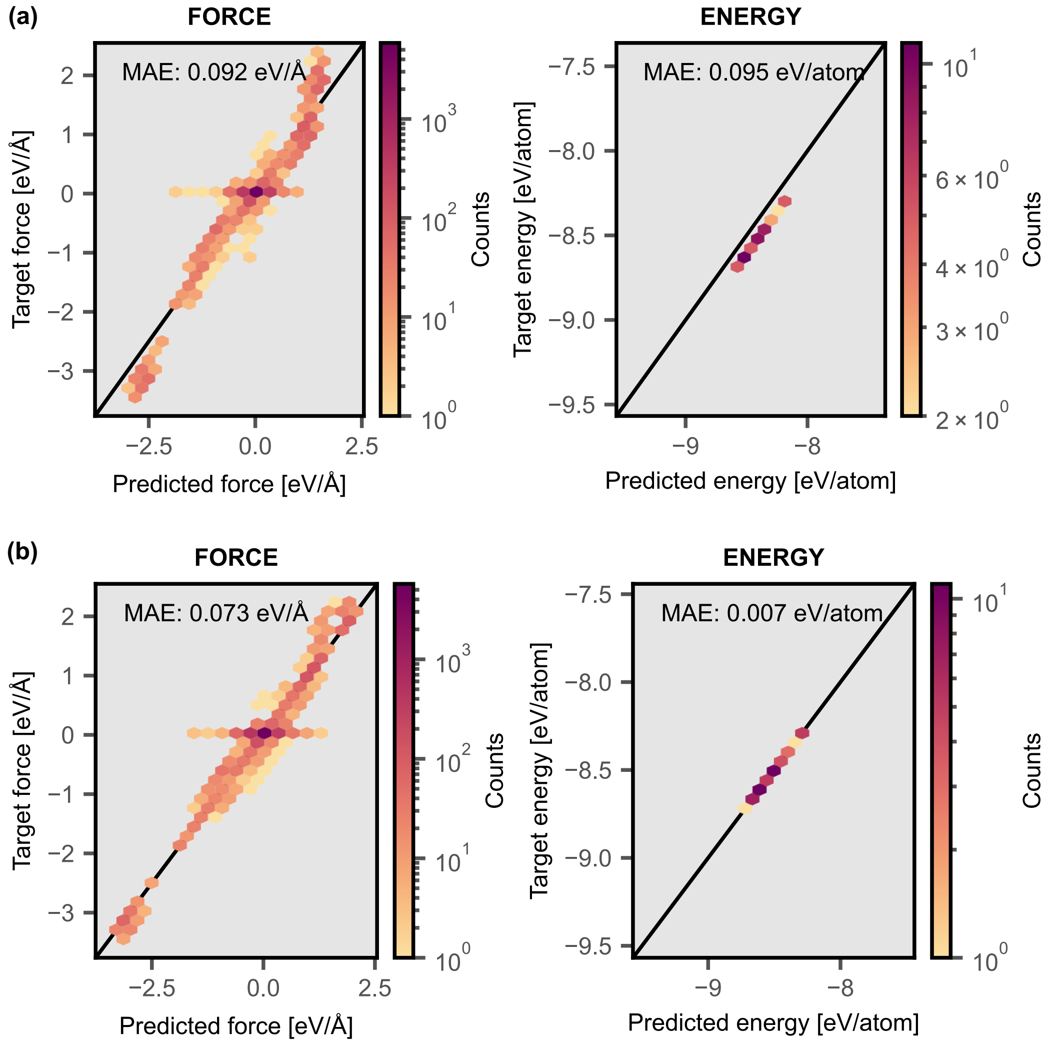


Figure S7: **NFF performance comparison for $LaMnO_3$(001) on the 47 handpicked surfaces.** (a) pre-trained CHGNet and (b) fine-tuned CHGNet.

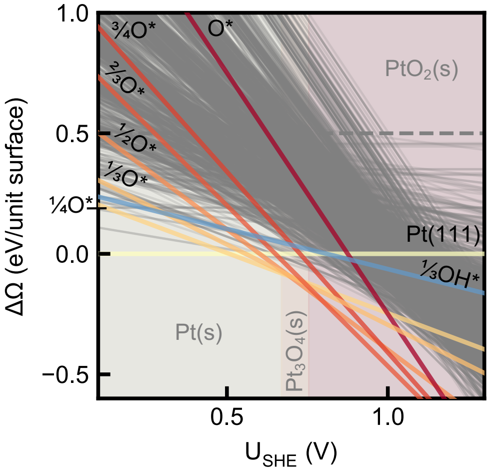


Figure S8: **Pt(111) energy analysis including additional sampled structures in gray.** $\Delta\Omega_{\mathrm{slab}}(U_{\mathrm{SHE}}, \mathrm{pH})$ with respect to the pristine surface in eV/surface unit cell of hand-picked and VSSR-MC sampled structures evaluated with fine-tuned MACE energies across $U_{\mathrm{SHE}}$ at fixed pH = 0.

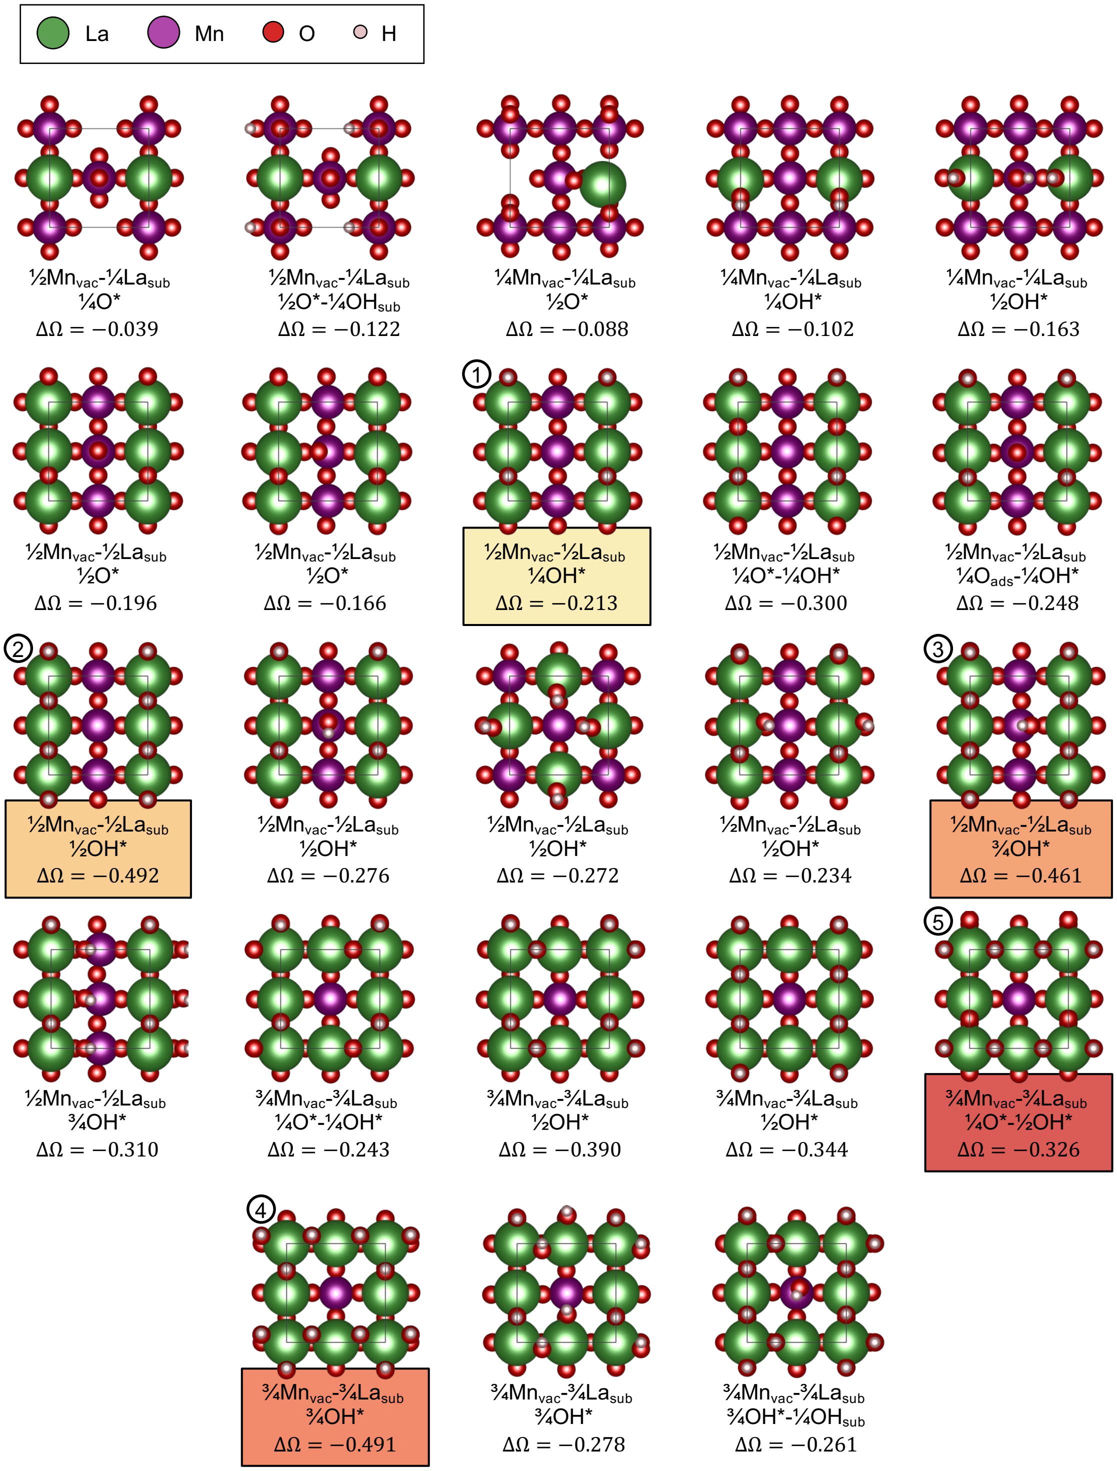


Figure S9: **Sampled mixed termination $LaMnO_3$(001) surfaces more stable than $MnO_2$-$\frac{1}{4}$OH* at $U_{SHE}$ = 0.6 V, pH = 12.** $\Delta\Omega_{slab}(U_{SHE}, \text{pH})$ energies are evaluated at the DFT level with respect to $MnO_2$-$\frac{1}{4}$OH* in eV/surface unit cell. Highlighted surfaces correspond to stable domains in Fig. 4(b-c).

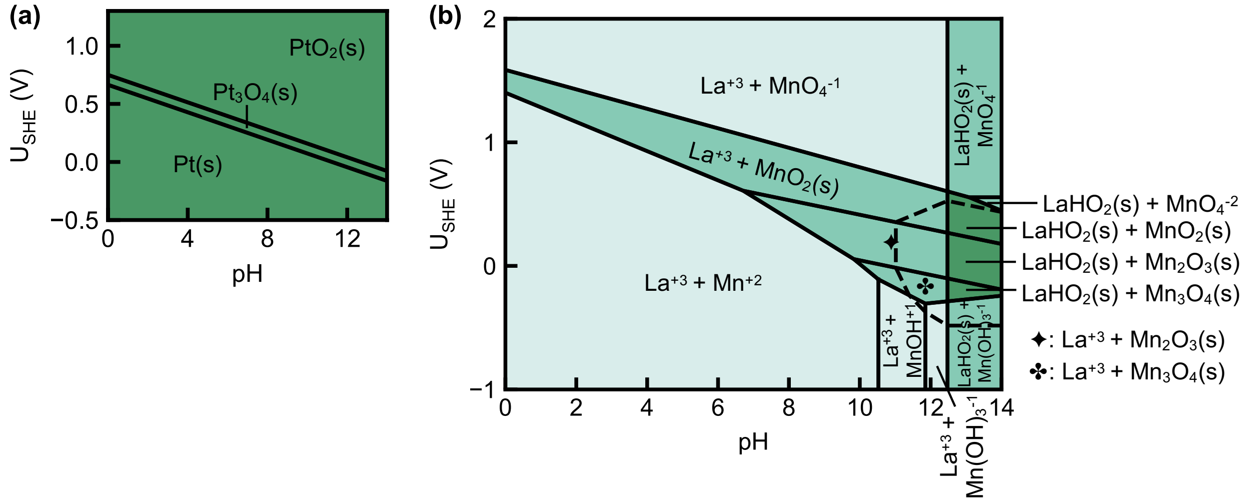


Figure S10: **Species Pourbaix diagrams of (a) Pt and (b) $LaMnO_3$ at $10^{-6}$ M dissolved species concentrations annotated with the stable solid or dissolved species at each combination of pH and $U_{SHE}$.** Solid species are in dark green, dissolved species are in pale blue, while mixed species are in teal. The bulk stability region for $LaMnO_3$ is encircled by dashed lines to reveal the underlying La and Mn species used in VSSR-MC sampling.

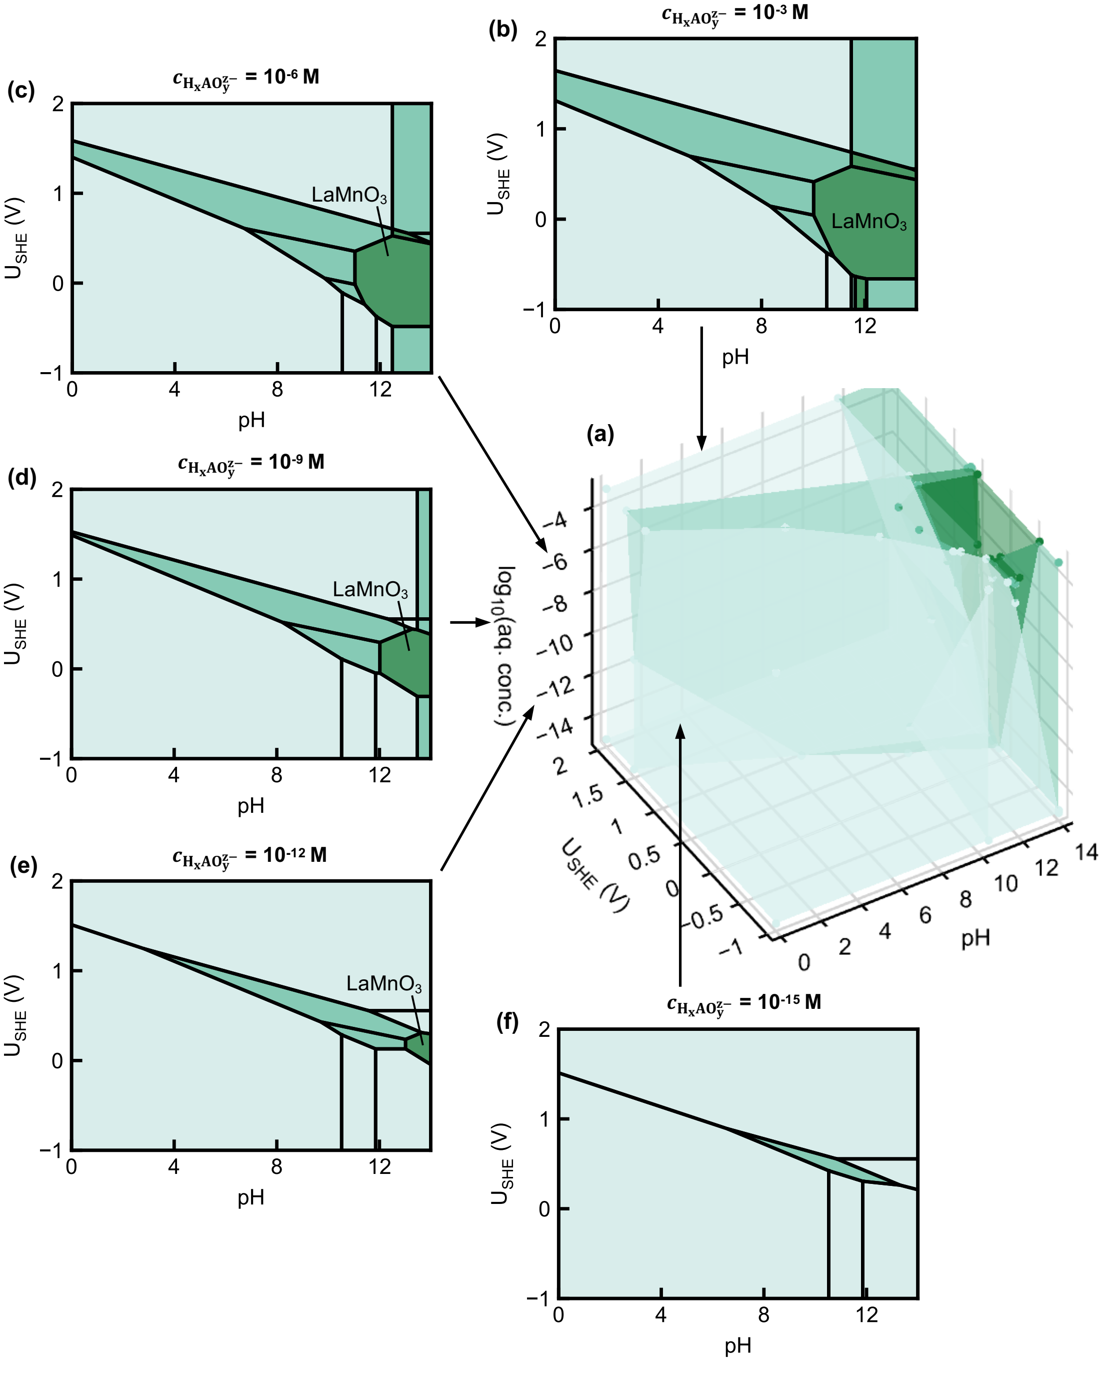


Figure S11: **pH-$U_{\mathbf{SHE}}$-$\log_{10} c_{H_xAO_y^{z-}}$ 3D species Pourbaix diagram and pH-$U_{\mathbf{SHE}}$ 2D slices at fixed $\log_{10} c_{H_xAO_y^{z-}}$ plotted with $LaMnO_3$ bulk stability region. Solid species are in dark green, dissolved species are in pale blue, while mixed species are in teal.** (a) 3D species Pourbaix diagram. 2D slices are extracted at $c_{H_xAO_y^{z-}}$ = (b) $10^{-3}$ M, (c) $10^{-6}$ M, (d) $10^{-9}$ M, (e) $10^{-12}$ M, and (f) $10^{-15}$ M.

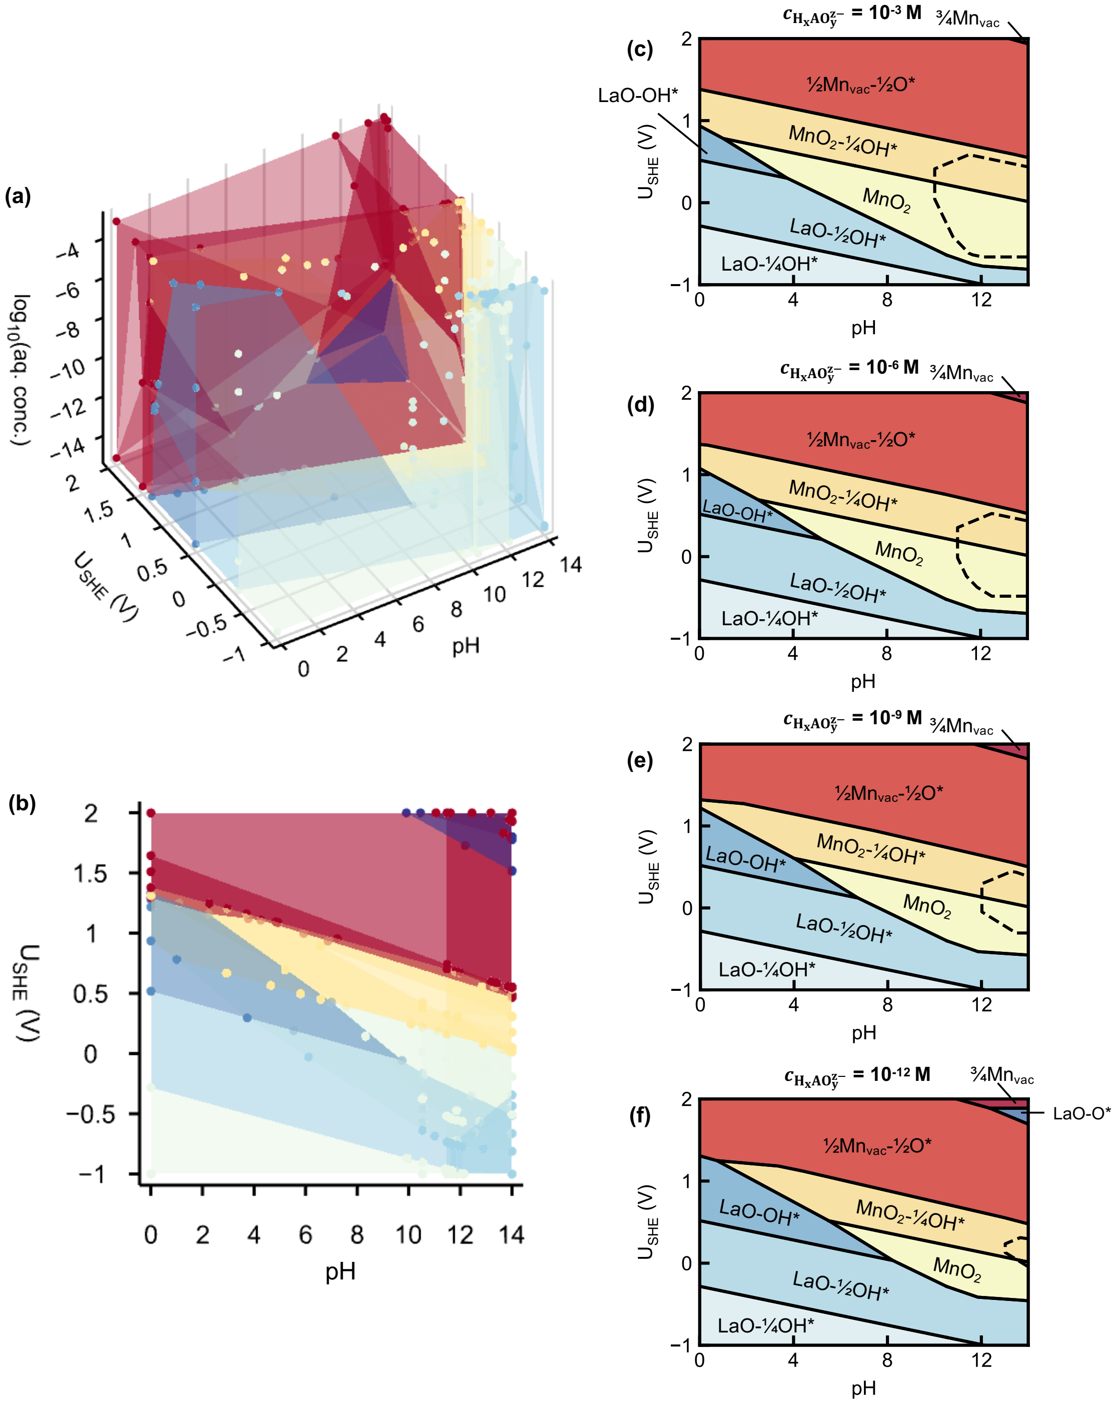


Figure S12: **pH-$U_{\mathbf{SHE}}$-$\log_{10} c_{\mathrm{H_xAO_y^{z-}}}$ 3D surface Pourbaix diagram with literature surfaces and pH-$U_{\mathbf{SHE}}$ 2D slices at fixed $c_{\mathrm{H_xAO_y^{z-}}}$ plotted with $\mathbf{LaMnO_3}$ bulk stability region enclosed by the dashed lines. Pristine surfaces are in light shades while more oxidized phases appear darker.** (a) 3D surface Pourbaix diagram. (b) 2D projection of surface Pourbaix diagram from high $c_{\mathrm{H_xAO_y^{z-}}}$. 2D slices are extracted at $c_{\mathrm{H_xAO_y^{z-}}} =$ (c) $10^{-3}$ M, (d) $10^{-6}$ M, (e) $10^{-9}$ M, and (f) $10^{-12}$ M.

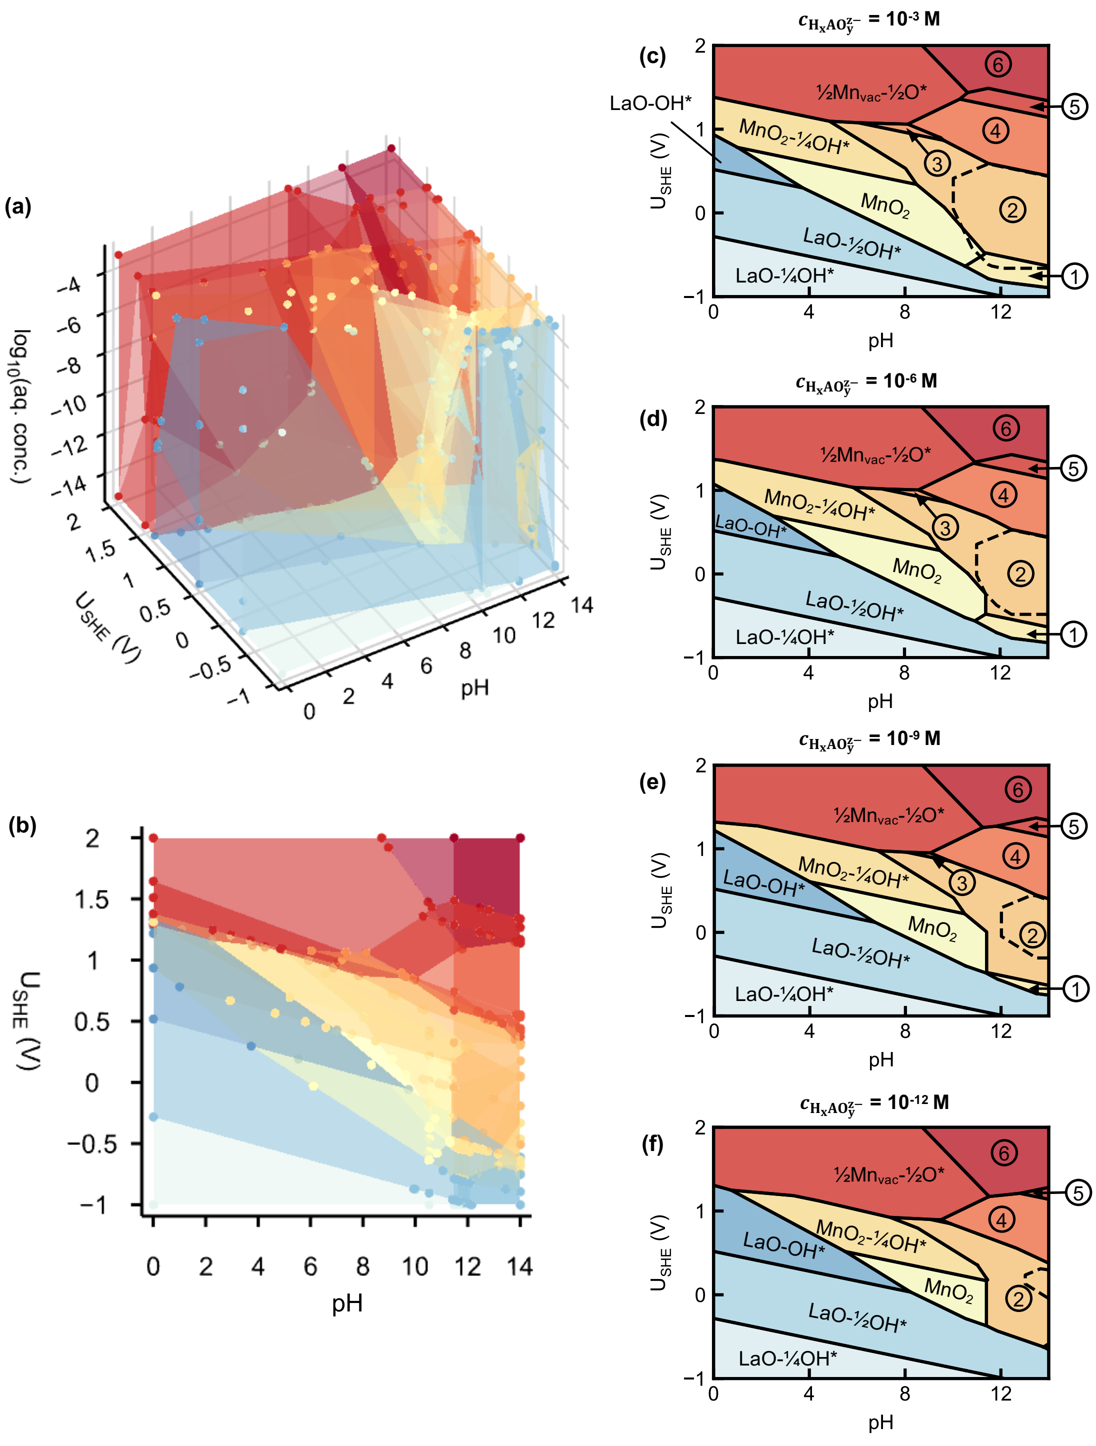


Figure S13: **pH-$U_{\mathrm{SHE}}$-$\log_{10} c_{\mathrm{H_xAO_y^{z-}}}$ 3D surface Pourbaix diagram with literature and additional sampled surfaces, and pH-$U_{\mathrm{SHE}}$ 2D slices at fixed $c_{\mathrm{H_xAO_y^{z-}}}$ plotted with $LaMnO_3$ bulk stability region enclosed by the dashed lines. Pristine surfaces are in light shades while more oxidized phases appear darker.** (a) 3D surface Pourbaix diagram. (b) 2D projection of surface Pourbaix diagram from high $c_{\mathrm{H_xAO_y^{z-}}}$. 2D slices are extracted at $c_{\mathrm{H_xAO_y^{z-}}}$ = (c) $10^{-3}$ M, (d) $10^{-6}$ M, (e) $10^{-9}$ M, and (f) $10^{-12}$ M. The numbered phases correspond to the sampled surfaces in Fig. 4(c).

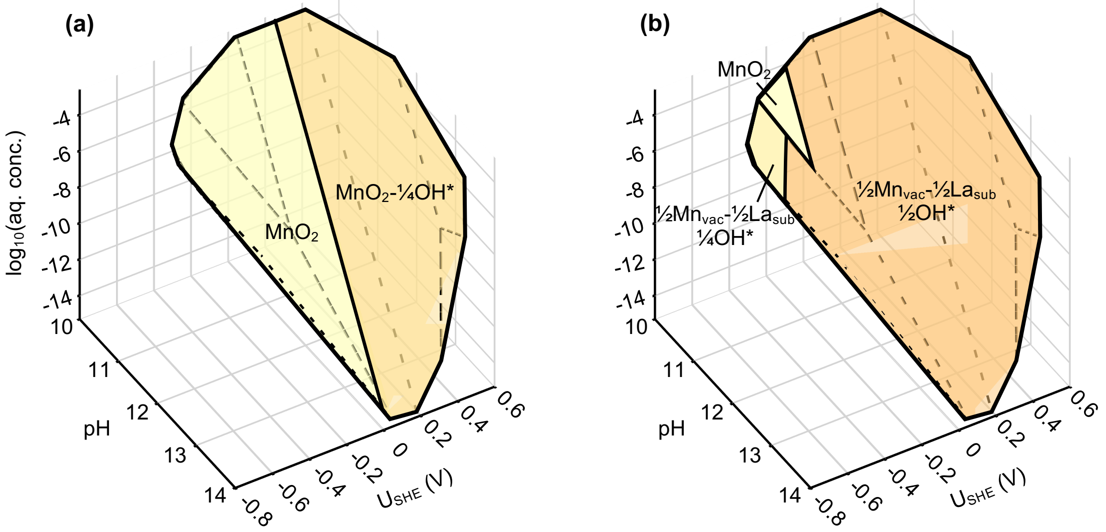


Figure S14: **3D perspectives of surface Pourbaix diagrams at thermodynamic equilibrium in the pH-$U_{\mathbf{SHE}}$-$\log_{10} c_{\mathrm{H_xAO_y^{z-}}}$ axes. More oxidized phases appear darker.** (a) surface Pourbaix diagram with literature surfaces. (d) surface Pourbaix diagram with literature and additional sampled surfaces.

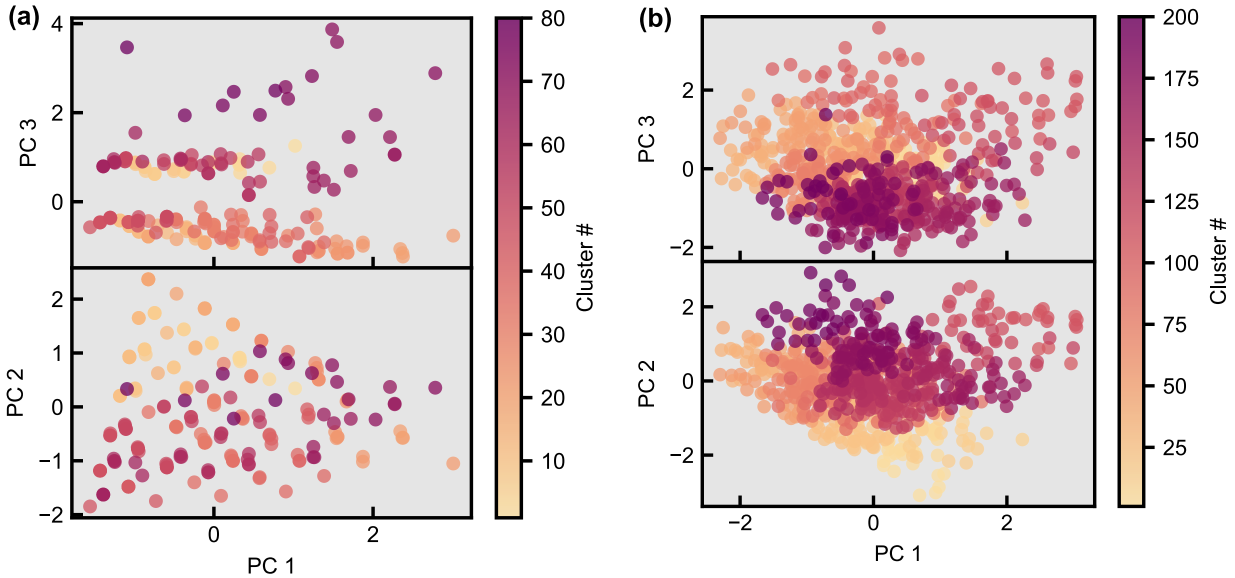


Figure S15: **Clustering of VSSR-MC structures using NFF embeddings visualized using the first 3 PCs.** (a) $(\sqrt{3} \times 3)$R30° Pt(111), (b) $2 \times 2$ $LaMnO_3$(001).

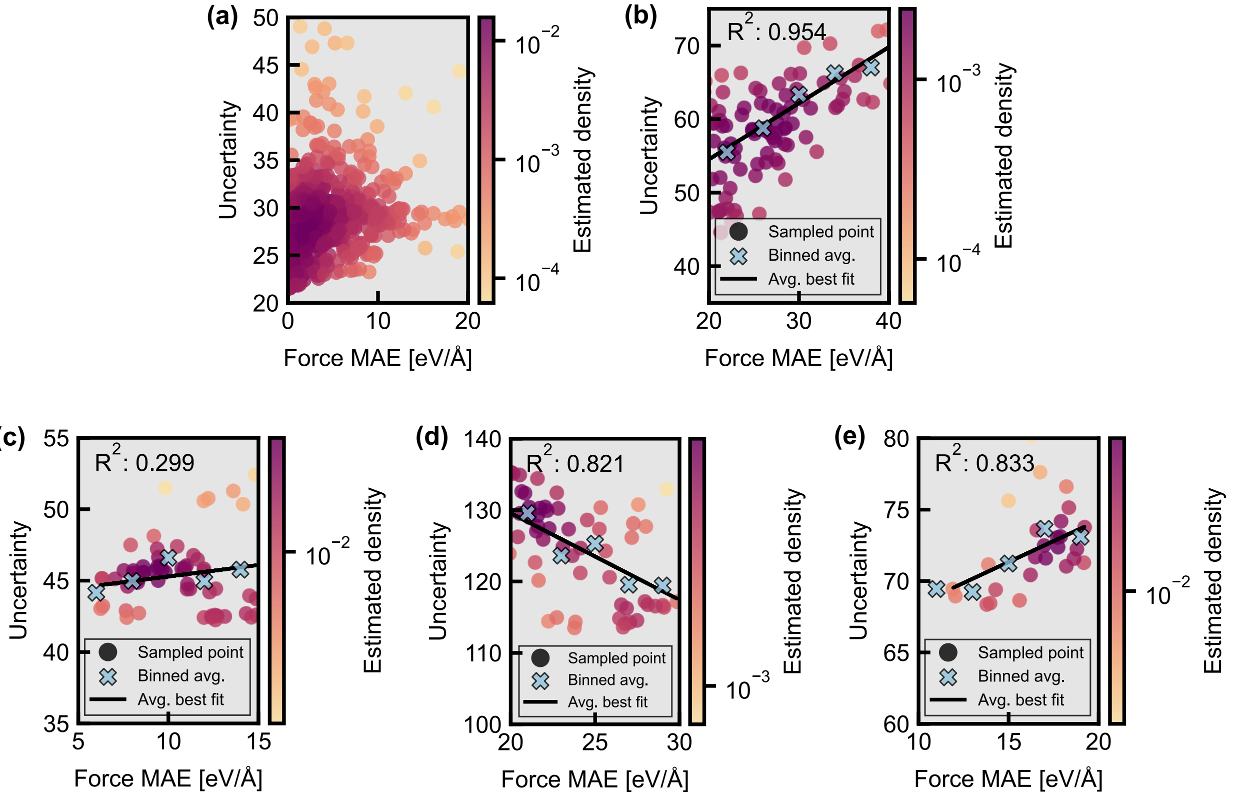


Figure S16: **GMM uncertainty calibration and result plots.** (a) Calibration with a subset of 5000 structures from MPtrj.[5] The calibration performance is commensurate with previous work.[6,7] (b) $2 \times 2$ $LaMnO_3(001)$ fine-tuning dataset and (c-e) $2 \times 2$, $3 \times 3$, and $\sqrt{3} \times 3$ Pt(111) fine-tuning datasets. (b) and (e) showed good positive correlation between estimated uncertainty and force MAE. (c) showed a lower correlation while (d) showed a negative correlation, which could be due to both the relatively low-data regime and Pt(111) with O*/OH* being more out of distribution with respect to the MPtrj dataset compared with $LaMnO_3(001)$ surfaces.

## References


(1) Hansen, H. A.; Rossmeisl, J.; Nørskov, J. K. Surface Pourbaix diagrams and oxygen reduction activity of Pt, Ag and Ni(111) surfaces studied by DFT. *Physical Chemistry Chemical Physics* **2008**, *10*, 3722–3730, Publisher: The Royal Society of Chemistry.

(2) Vinogradova, O.; Krishnamurthy, D.; Pande, V.; Viswanathan, V. Quantifying Confidence in DFT-Predicted Surface Pourbaix Diagrams of Transition-Metal Electrode–Electrolyte Interfaces. *Langmuir* **2018**, *34*, 12259–12269, Publisher: American Chemical Society.

(3) Rong, X.; Kolpak, A. M. Ab Initio Approach for Prediction of Oxide Surface Structure, Stoichiometry, and Electrocatalytic Activity in Aqueous Solution. *The Journal of Physical Chemistry Letters* **2015**, *6*, 1785–1789.

(4) Du, X. Data for: Accelerating and enhancing thermodynamic simulations of electrochemical interfaces. 2025; `https://doi.org/10.5281/zenodo.15066440`.

(5) Deng, B. Materials Project Trajectory (MPtrj) Dataset. 2023; `https://figshare.com/articles/dataset/Materials_Project_Trjectory_MPtrj_Dataset/23713842/2`.

(6) Zhu, A.; Batzner, S.; Musaelian, A.; Kozinsky, B. Fast uncertainty estimates in deep learning interatomic potentials. *The Journal of Chemical Physics* **2023**, *158*, 164111.

(7) Tan, A. R.; Urata, S.; Goldman, S.; Dietschreit, J. C. B.; Gómez-Bombarelli, R. Single-model uncertainty quantification in neural network potentials does not consistently outperform model ensembles. *npj Computational Materials* **2023**, *9*, 1–11, Publisher: Nature Publishing Group.
